# Supplementary material for: Tensor Processing Units for Financial Monte Carlo
Source: arXiv:1906.02818 source file (2020-01-27)
Supplement: Supplementary file 1 [file appendix.tex]

\subsubsection{Replicating portfolio and Risk Neutral probability}
Portfolio theory and no-arbitrage arguments from 1969-1973 constitute the cornerstone of the application of stochastic processes to quantitative finance for which Fisher Black, Myron Scholes and Robert Merton would eventually win the Novel Prize economics in 1997.
European option pricing is a simple introductory case for the corresponding concepts.
Consider a uni-dimensional process $(X_t)$ modeling the price of an asset whose dynamics follow Equation~\ref{eq:SDE}, a European option is defined as a derivative that will give the owner of the contract a Payoff $f(X_T)$ at an ulterior date $T$.
The pricing problem considers determining the price $g(X_0)$ of such an option at $t=0$ under the no-arbitrage principle.
In an insurance setting, in the absence of the possibility to hedge against the contingencies affecting $(X_t)$ between $0$ and $T$, 
the answer would simply that the price of the contract is simply $E_{\mathbb{P}}[X_T]$.
However, if the underlying to the contract is a liquid asset (e.g. traded equity, bond or commodity),
it is possible for the seller of the contract to hedge his position thanks to a \emph{replicating portfolio} consisting of a risk-free asset (e.g. cash) and the underlying $(X_t)$ in proportions that need to be constantly adjusted as $(X_t)$ evolves between $0$ and $T$.
Assuming such a portfolio can be derived, the no-arbitrage principle stipulates that the price of the option is non other than the cost needed to initialize the adaptive portfolio.

\subsubsection{Derivatives pricing and sensitivity analysis}
Delineating the details of the corresponding portfolio is out of the scope out the present paper.
However we will just bring to the fore two key results whose ramifications are tremendous for Monte Carlo methods:
\begin{itemize}
    \item A Cameron-Martin change of measure shows that there exists another probability distribution $\mathbb{Q}$ whose Radon-Nikodim derivative $\frac{d\mathbb{Q}}{d\mathbb{P}}$ w.r.t. $\mathbb{P}$ can be derived such that the price of a European contract is $g(X_0)=E_{\mathbb{Q}} \left[ X_T \right]$. The change of measure from the historical probability measure to the risk-free measure reflects the ability to hedge by synthesizing a replicating portfolio whose value at $T$ is exactly that of the payoff.
    \item The quantity of the underlying that should be held at any time $t$ to produce the replicating portfolio and hedge the option is exactly the ``Delta'' of the option, i.e. the first order derivative $\nabla_{X_0} g(X_0)$. Such a property introduces sensitivity analysis as a key aspect of quantitative finance. First and second order sensitivities are also routinely computed w.r.t. to other parameters in dynamical models to compute the exposure to the different factors underlying the model (e.g. volatility, interest rate etc.). Under some conditions, 
    $\nabla_{\theta} g_{\theta}(X_0) = \nabla_{\theta} E_{\mathbb{Q}} \left[X_T\right] = E_{\mathbb{Q}} \left[\nabla_{\theta} X_T\right]$.
\end{itemize}
Those statements imply that estimating expectations can be a crucial tool to price derivatives, hedge them, compute exposures and generally provide risk assessment under the historical and risk-free probabilities.
Other pricing methods are also routinely uses such as analytic approximation formulas which for instance use Black-Scholes like formulae to infer prices by interpolation.
Partial Differential Equations for underlings that have a few degrees of freedom are routinely for fast pricing thanks to the Feynman-Kac formula but unfortunately do not scale well with $p$.
When underlying assets involve high dimensional correlated dynamics, Monte-Carlo methods remain the most competitive option in spite of their computational intensity.
